# Supplementary material for: Fire360: A Benchmark for Robust Perception and Episodic Memory in Degraded 360-Degree Firefighting Videos
Source: arXiv:2506.02167 source file (2025-06-02)
Supplement: Supplementary file 1 [file appendix-examples.tex]

1. Visual Question Answering (VQA)
Task Description (from Fire360): Measures spatial reasoning in 360° panoramic frames under degraded conditions, answering expert-authored questions about object presence, responder configuration, or protocol adherence.

\vspace{1mm}
\noindent \textit{Examples:} 
\begin{itemize}
\item ``Is the exit door visible through the smoke?'' $\rightarrow$ ``No, the door is occluded by dense smoke.''
\item ``Are responders maintaining a two-point contact on the ladder?'' $\rightarrow$ ``Yes, both hands are on the rails.''
\item ``Is the hose nozzle positioned toward the fire base?'' $\rightarrow$ ``No, it points above the flame.''
\item ``Is a civilian present behind the collapsed beam?'' $\rightarrow$ ``Yes, a civilian is partially visible.''
\end{itemize}
Rationale:

Safety Protocols: Two-point contact (NFPA 1001) and hose positioning reflect critical firefighting procedures.
Degradation: Smoke occlusion and collapsed beams emphasize low-visibility challenges.
Diversity: Questions cover spatial layout, protocol adherence, and object presence, aligning with the task’s scope.

2. Temporal Action Captioning
Task Description: Tests grounded descriptions of firefighter behavior in 10–20 second clips under degraded visibility, outputting natural language captions.

Examples:

\vspace{1mm}
\noindent \textit{Examples:} 
\begin{itemize}
\item Given a 10s clip of a firefighter crouching and breaking a window, output: ``Responder breaks glass to access burning room.''
\item Given a 15s clip of a team advancing through smoke, output: ``Responders crawl in single file to search for victims.''
\item Given a 12s clip of a firefighter adjusting PPE, output: ``Responder secures gas mask in low-visibility conditions.''
\item Given a 20s clip of ladder positioning, output: ``Team erects ladder to access second-story window.''
\end{itemize}

Rationale:

Safety Protocols: Crawling (NFPA 1410), PPE adjustment, and ladder use reflect standard procedures.
Degradation: Smoke and low-visibility conditions test temporal understanding in chaotic scenes.
Diversity: Captions cover access, search, PPE, and structural tasks, capturing varied actions.

3. Object Localization under Distortion
Task Description: Evaluates object detection robustness under occlusion and thermal blur in 360° imagery, localizing gear (e.g., SCBA tanks, helmets) with IoU > 0.5.

Examples:

\vspace{1mm}
\noindent \textit{Examples:} 
\begin{itemize}
\item Localize an SCBA tank in a smoke-obscured hallway; success if IoU $> 0.5$ with expert-verified region.
\item Detect a firefighter helmet amidst thermal distortion near a fire source; success if IoU $> 0.5$.
\item Identify a hose nozzle in a low-light, debris-cluttered room; success if IoU $> 0.5$.
\item Locate a gas mask dropped in a smoke-filled corridor; success if IoU $> 0.5$.
\end{itemize}

Rationale:

Safety Protocols: SCBA tanks, helmets, and gas masks are critical PPE (NFPA 1851); hoses are essential for suppression.
Degradation: Smoke, thermal distortion, and low light test localization robustness.
Diversity: Examples cover different gear types and environmental challenges.

4. Safety-Critical Reasoning
Task Description: Identifies violations of standard safety procedures in static frames or video segments, outputting “safe” or “unsafe” with justifications.

Examples:

\vspace{1mm}
\noindent \textit{Examples:} 
\begin{itemize}
\item Prompt: ``Assess the responder’s ladder use.'' $\rightarrow$ ``Unsafe: The responder lacks a second point of contact.''
\item Prompt: ``Evaluate PPE compliance in the fire zone.'' $\rightarrow$ ``Unsafe: The responder’s gas mask is not sealed.''
\item Prompt: ``Check the hose operation technique.'' $\rightarrow$ ``Safe: The nozzle is aimed at the fire base.''
\item Prompt: ``Assess team formation in smoke.'' $\rightarrow$ ``Unsafe: Responders are not maintaining visual contact.''
\end{itemize}

Rationale:

Safety Protocols: Two-point contact, PPE sealing (NFPA 1500), hose aiming, and team contact (NFPA 1710) are core procedures.
Degradation: Smoke and fire zones emphasize protocol adherence under stress.
Diversity: Examples cover structural, PPE, suppression, and team coordination violations.

5. Transformed Object Retrieval (TOR)
Task Description: Matches a pristine object exemplar to its fire-damaged counterpart in an unpaired 360° scene, testing transformation-invariant recognition.

Examples:

latex

Copy
\vspace{1mm}
\noindent \textit{Examples:} 
\begin{itemize}
\item Given a pristine red firefighter helmet, locate its melted, soot-covered version near a collapsed beam; success if IoU $> 0.5$.
\item Given a clean SCBA tank, identify its charred, deformed version in a smoke-filled room; success if IoU $> 0.5$.
\item Given an intact hose nozzle, find its warped, ash-covered counterpart near a burnt wall; success if IoU $> 0.5$.
\end{itemize}
Rationale:

Safety Protocols: Helmets, SCBA tanks, and nozzles are critical gear; recognizing damaged versions ensures operational continuity.
Degradation: Melting, charring, and smoke test material reasoning and memory.
Diversity: Examples cover rigid (SCBA) and deformable (hose) objects in varied contexts.
