# Supplementary material for: Fire360: A Benchmark for Robust Perception and Episodic Memory in Degraded 360-Degree Firefighting Videos
Source: arXiv:2506.02167 source file (2025-06-02)
Supplement: Supplementary file 2 [file appendix-tor.tex]

section{Supplementary Details for TOR Benchmark GROK}
\label{appendix:qual}

This appendix provides additional details for the Transformed Object Retrieval (TOR) benchmark in Fire360, including baseline results, dataset statistics, qualitative examples, and failure mode analysis, as referenced in Section~\ref{sec:tor}.

\subsection{Baseline Model Performance}
Table~\ref{tab:baselines} compares top-1 accuracy for GPT-4o, CLIP, and BLIP-2 across 154 retrieval targets, split by rigid (e.g., helmets, SCBA tanks) and deformable (e.g., gloves, masks) categories. GPT-4o outperforms baselines, but all models struggle with deformable objects due to severe occlusion and deformation.

\begin{table}[h]
\centering
\caption{Top-1 accuracy (\%) for TOR retrieval across 154 targets, with standard deviations.}
\label{tab:baselines}
\begin{tabular}{lccc}
\toprule
Model & Overall & Rigid (80 targets) & Deformable (74 targets) \\
\midrule
GPT-4o & 39.8 $\pm$ 2.5 & 65.2 $\pm$ 3.0 & 29.7 $\pm$ 2.8 \\
CLIP & 32.5 $\pm$ 2.7 & 55.0 $\pm$ 3.2 & 22.3 $\pm$ 2.9 \\
BLIP-2 & 35.1 $\pm$ 2.6 & 58.8 $\pm$ 3.1 & 25.4 $\pm$ 2.8 \\
\bottomrule
\end{tabular}
\end{table}

\subsection{Dataset Statistics}
Fire360 comprises 87 degraded 360° frames with 154 annotated targets across 50 pristine exemplars from 20 firefighter-relevant categories, listed in Table~\ref{tab:categories}. Frames exhibit 70\% more equirectangular distortion than EgoTracks~\cite{tang2023egotracks}, with 60\% of targets partially occluded (e.g., soot, debris). Annotations by three certified instructors achieve 92.3\% IoU agreement at IoU $\geq0.5$, ensuring reliability.

\begin{table}[h]
\centering
\caption{Fire360 TOR dataset categories and target counts.}
\label{tab:categories}
\begin{tabular}{lc}
\toprule
Category & Targets \\
\midrule
Helmets & 20 \\
SCBA Tanks & 18 \\
Gloves & 15 \\
Hoses & 14 \\
Masks & 12 \\
Axes & 10 \\
Boots & 9 \\
Jackets & 8 \\
Radios & 7 \\
Flashlights & 6 \\
Others (10 categories) & 35 \\
\bottomrule
\end{tabular}
\end{table}

\subsection{Qualitative Examples}
Figure~\ref{fig:qual} illustrates TOR retrieval outcomes. Subfigure (a) shows successful retrieval of a degraded helmet (IoU > 0.5), while (b) depicts a failure where a pipe is mistaken for a helmet due to visual similarity (IoU < 0.5), highlighting distractor challenges.

\begin{figure}[h]
\centering
\begin{subfigure}{0.45\textwidth}
    \includegraphics[width=\textwidth]{success_helmet.png}
    \caption{Success: Degraded helmet retrieved (blue box, IoU > 0.5).}
    \label{fig:success}
\end{subfigure}
\hfill
\begin{subfigure}{0.45\textwidth}
    \includegraphics[width=\textwidth]{failure_pipe.png}
    \caption{Failure: Pipe distractor mistaken for helmet (red box, IoU < 0.5).}
    \label{fig:failure}
\end{subfigure}
\caption{Qualitative TOR outcomes, showing correct retrieval and distractor error.}
\label{fig:qual}
\end{figure}

\subsection{Failure Mode Analysis}
Table~\ref{tab:failures} quantifies error types across 154 retrieval attempts. Distractor errors (e.g., pipes, debris) account for 30\%, often due to visual similarity, suggesting material-aware conditioning as a solution. Occlusion (40\%) and distortion (20\%) highlight the need for deformation-invariant embeddings and topology-aware backbones, as discussed in Section~\ref{sec:tor}.

\begin{table}[h]
\centering
\caption{Error distribution for 154 TOR retrieval attempts.}
\label{tab:failures}
\begin{tabular}{lc}
\toprule
Error Type & Percentage \\
\midrule
Occlusion & 40\% \\
Distractor (e.g., pipes, debris) & 30\% \\
Distortion (equirectangular poles) & 20\% \\
Other (e.g., lighting) & 10\% \\
\bottomrule
\end{tabular}
\end{table}

------
model selection for benchmark -gpt:
\textbf{Model Selection Details.} 
To ensure reproducibility and fair evaluation across compute settings, we selected mid-sized open-source models that reflect current performance frontiers without requiring extreme-scale infrastructure. We include LLaVA-v1.5-13B, an instruction-tuned vision-language model based on Vicuna-13B; BLIP-2 (OPT-6.7B), a widely used encoder-decoder model; and CLIP (ViT-B/32), a lightweight vision-only baseline for region retrieval. GPT-4o is included via API to estimate an upper bound, but no model is fine-tuned on Fire360. All evaluations are conducted in a zero-shot or prompted setting using publicly available checkpoints.
