# Supplementary material for: Fire360: A Benchmark for Robust Perception and Episodic Memory in Degraded 360-Degree Firefighting Videos
Source: arXiv:2506.02167 source file (2025-06-02)
Supplement: Supplementary file 3 [file appendix.tex]

\appendix
\section*{Appendix}

\subsection{Model Setup and Evaluation Protocols}
\label{appendix:modelsetup}

All evaluations operate in a zero-shot or prompted setting, with no fine-tuning on Fire360. This setup reflects real-world deployment conditions where models must generalize to unseen, degraded inputs. We benchmark both proprietary and open-source vision-language models to capture a broad spectrum of architectural design and training strategies. GPT-4o is accessed via the OpenAI API (May 2025 snapshot) with decoding parameters set to temperature = 0.7 and top-p = 0.95. Task-specific prompts and invocation formats appear in Appendix~\ref{appendix:qual}.

\textbf{Model Selection.} GPT-4o is included for its strong multimodal reasoning capabilities. LLaVA-v1.5-13B (based on Vicuna-13B), BLIP-2 (OPT-6.7B), and Qwen-VL-Chat (7B) represent publicly available vision-language models with diverse instruction tuning protocols. CLIP (ViT-B/32) serves as a baseline for the Transformed Object Retrieval (TOR) task due to its widespread use in image-text embedding alignment. Grounding DINO (v1) generates bounding box proposals for detection and retrieval, producing an average of 36.2 regions per frame at a confidence threshold of 0.4, followed by non-maximum suppression (IoU = 0.3). For temporal captioning, we evaluate GLaMM-7B as a representative model for generating language under visual degradation.

\textbf{Evaluation Metrics.} Each task uses a standard yet degradation-sensitive metric. TOR performance is measured using top-1 retrieval accuracy with an IoU threshold of 0.5. Visual Question Answering (VQA) uses exact match accuracy. Temporal Captioning is evaluated via BLEU-4 to quantify surface-level linguistic agreement. Safety-Critical Reasoning uses binary checklist accuracy based on domain-verified procedural outputs.

\textbf{Data Splits and Runtime.} The dataset is split into 60\% training (137 videos), 20\% validation (45 videos), and 20\% test (46 videos), stratified by degradation level, lighting, and procedural diversity. All experiments run on NVIDIA A100 GPUs (40GB). TOR inference across 154 targets requires approximately 2.5 GPU-hours (batch size 16); CLIP-based retrieval completes in 45 minutes. Preprocessing uses OpenCV to convert equirectangular frames into 90$^\circ$ rectilinear projections.

\subsection{Stratified Performance and Statistical Analysis}
\label{appendix:stats}

Fire360's equirectangular panoramas introduce non-uniform spatial distortion, particularly near the top and bottom edges of each frame. This distortion arises from the spherical-to-rectangular projection inherent to 360$^\circ$ imagery. Empirically, distortion near polar regions increases by approximately 70\% compared to equatorial zones~\cite{shi2023panovpr}, negatively impacting object localization and retrieval accuracy in peripheral image areas. Figure~\ref{fig:distortion_zones} visualizes this effect: the green bounding box indicates a region with minimal distortion, while the red box marks areas of maximal projection artifacts, often near the poles or lower image boundary.

\begin{figure}[h]
\centering
\includegraphics[width=\textwidth]{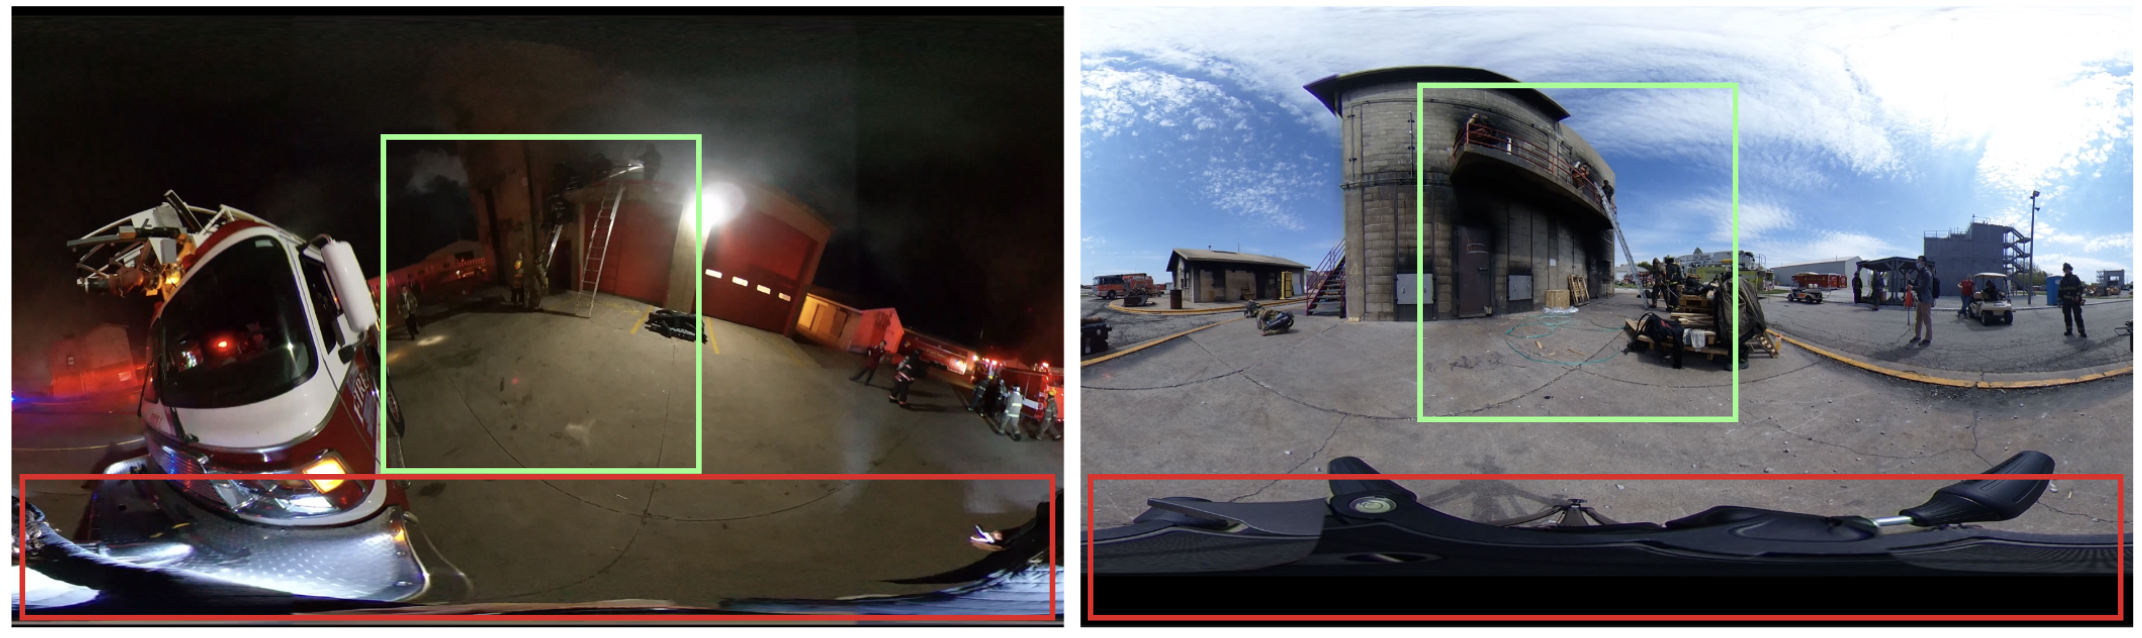}
\caption{Illustration of distortion severity in Fire360's equirectangular projections. Green regions exhibit low distortion and preserve geometric structure, while red regions show significant stretching, especially at the vertical extremes. These artifacts degrade both object localization and retrieval accuracy.}
\label{fig:distortion_zones}
\end{figure}

To analyze model-level failure modes, we examine the dominant sources of error in the Transformed Object Retrieval (TOR) task across $n=154$ annotated instances. Table~\ref{tab:tor_failure_summary} summarizes the error distribution. Distractor regions—e.g., metallic pipes or ladders visually similar to helmets—account for 30\% of failures. Occlusion, especially from smoke, accounts for another 25\%. Material confusion, where models struggle to differentiate between similarly shaped objects with different material cues (e.g., plastic vs. metal), contributes 20\% of the total error.

To quantify model robustness, we report 95\% bootstrap confidence intervals over 1{,}000 resamples for TOR accuracy (Table~\ref{tab:tor_ci}). GPT-4o achieves the highest average performance but still demonstrates significant variance under distortion and occlusion. BLIP-2 and CLIP perform comparably, with narrower confidence bands reflecting overall lower accuracy.

\begin{table}[t]
\centering
\caption{TOR model performance and failure attribution. The dominant error for each model is shown alongside its contribution to overall failures across $n=154$ targets.}
\label{tab:tor_failure_summary}
\footnotesize
\resizebox{\linewidth}{!}{
\begin{tabular}{@{}c@{}}
\begin{tabular}{lccc}
\toprule
\textbf{Model} & \textbf{Top-1 Accuracy} & \textbf{Dominant Error Type} & \textbf{Error Prevalence (Global)} \\
\midrule
GPT-4o & 39.8\% & Visual distractors (e.g., pipes, ladders) & 30\% \\
BLIP-2 & 35.1\% & Material confusion (e.g., plastic vs. metal) & 20\% \\
CLIP & 32.5\% & Occlusion (e.g., smoke, debris) & 25\% \\
\bottomrule
\end{tabular}
\end{tabular}
}
\end{table}
\begin{table}[t]
\centering
\caption{95\% confidence intervals for TOR retrieval accuracy (IoU $\geq$ 0.5, $n=154$).}
\label{tab:tor_ci}
\footnotesize
\resizebox{0.4\linewidth}{!}{
\begin{tabular}{@{}c@{}}
\begin{tabular}{lcc}
\toprule
\textbf{Model} & \textbf{Lower Bound} & \textbf{Upper Bound} \\
\midrule
GPT-4o & 37.6\% & 42.2\% \\
BLIP-2 & 32.8\% & 37.4\% \\
CLIP & 30.3\% & 34.9\% \\
\bottomrule
\end{tabular}
\end{tabular}
}
\end{table}

Finally, we observe a strong correlation between failures in spatial reasoning and memory-based retrieval. VQA performance in high-degradation scenes (e.g., dense smoke or poor lighting) drops to 9.8\%, and this degradation correlates with TOR error rates (Pearson $r = 0.72$), suggesting that both tasks are jointly limited by failures in visual grounding under uncertainty.

\subsection{Toolkit Structure}
\label{appendix:toolkit}

The Fire360 benchmark toolkit is designed to support reproducible evaluation across all five tasks. It includes preprocessing utilities, evaluation scripts, and standardized input-output formats, and will be released publicly upon acceptance.

Preprocessing is performed using OpenCV, which converts equirectangular panoramas to 90$^\circ$ rectilinear projections. Frame resizing is applied according to model-specific requirements: CLIP operates on 224$\times$224 crops, while GPT-4o uses 512$\times$512 inputs. 

The evaluation suite includes task-specific scorers: exact match accuracy for VQA, mean IoU evaluation for TOR, BLEU-4 scoring for temporal captioning, and binary checklist comparison for safety-critical reasoning. Each script is designed to run independently on individual frames or video clips, and supports batch-mode evaluation on the test split.

All inputs are formatted in JSON, containing file paths, model prompts, and configuration parameters. Evaluation outputs are stored in CSV files with predicted labels, metrics, and confidence scores.

Full test-time evaluation of the benchmark requires approximately 4 GPU-hours on NVIDIA A40s, or 2.5 hours on A100s. The dataset, including raw video files and annotations, occupies approximately 400GB of storage.

\subsection{Annotation Tool and Schema}
\label{appendix:annotationtool}

To support structured labeling of degraded 360$^\circ$ firefighter footage, we provide a browser-based annotation interface designed for equirectangular and rectilinear projections. The interface enables frame-level labeling for actions, objects, and scene conditions, with support for transformation tracking and environmental metadata. Figures~\ref{fig:annotation_tool_ui} and~\ref{fig:annotation_modes} illustrate the Fire360 annotation interface. Figure~\ref{fig:annotation_tool_ui} shows the layout for selecting annotation types and defining object-level metadata, while Figure~\ref{fig:annotation_modes} presents detailed forms for action-level, environmental, and temporal sequence annotations. We plan to release the tool publicly to support extensibility and custom workflows.

\begin{figure}[h]
\centering
\includegraphics[width=\textwidth]{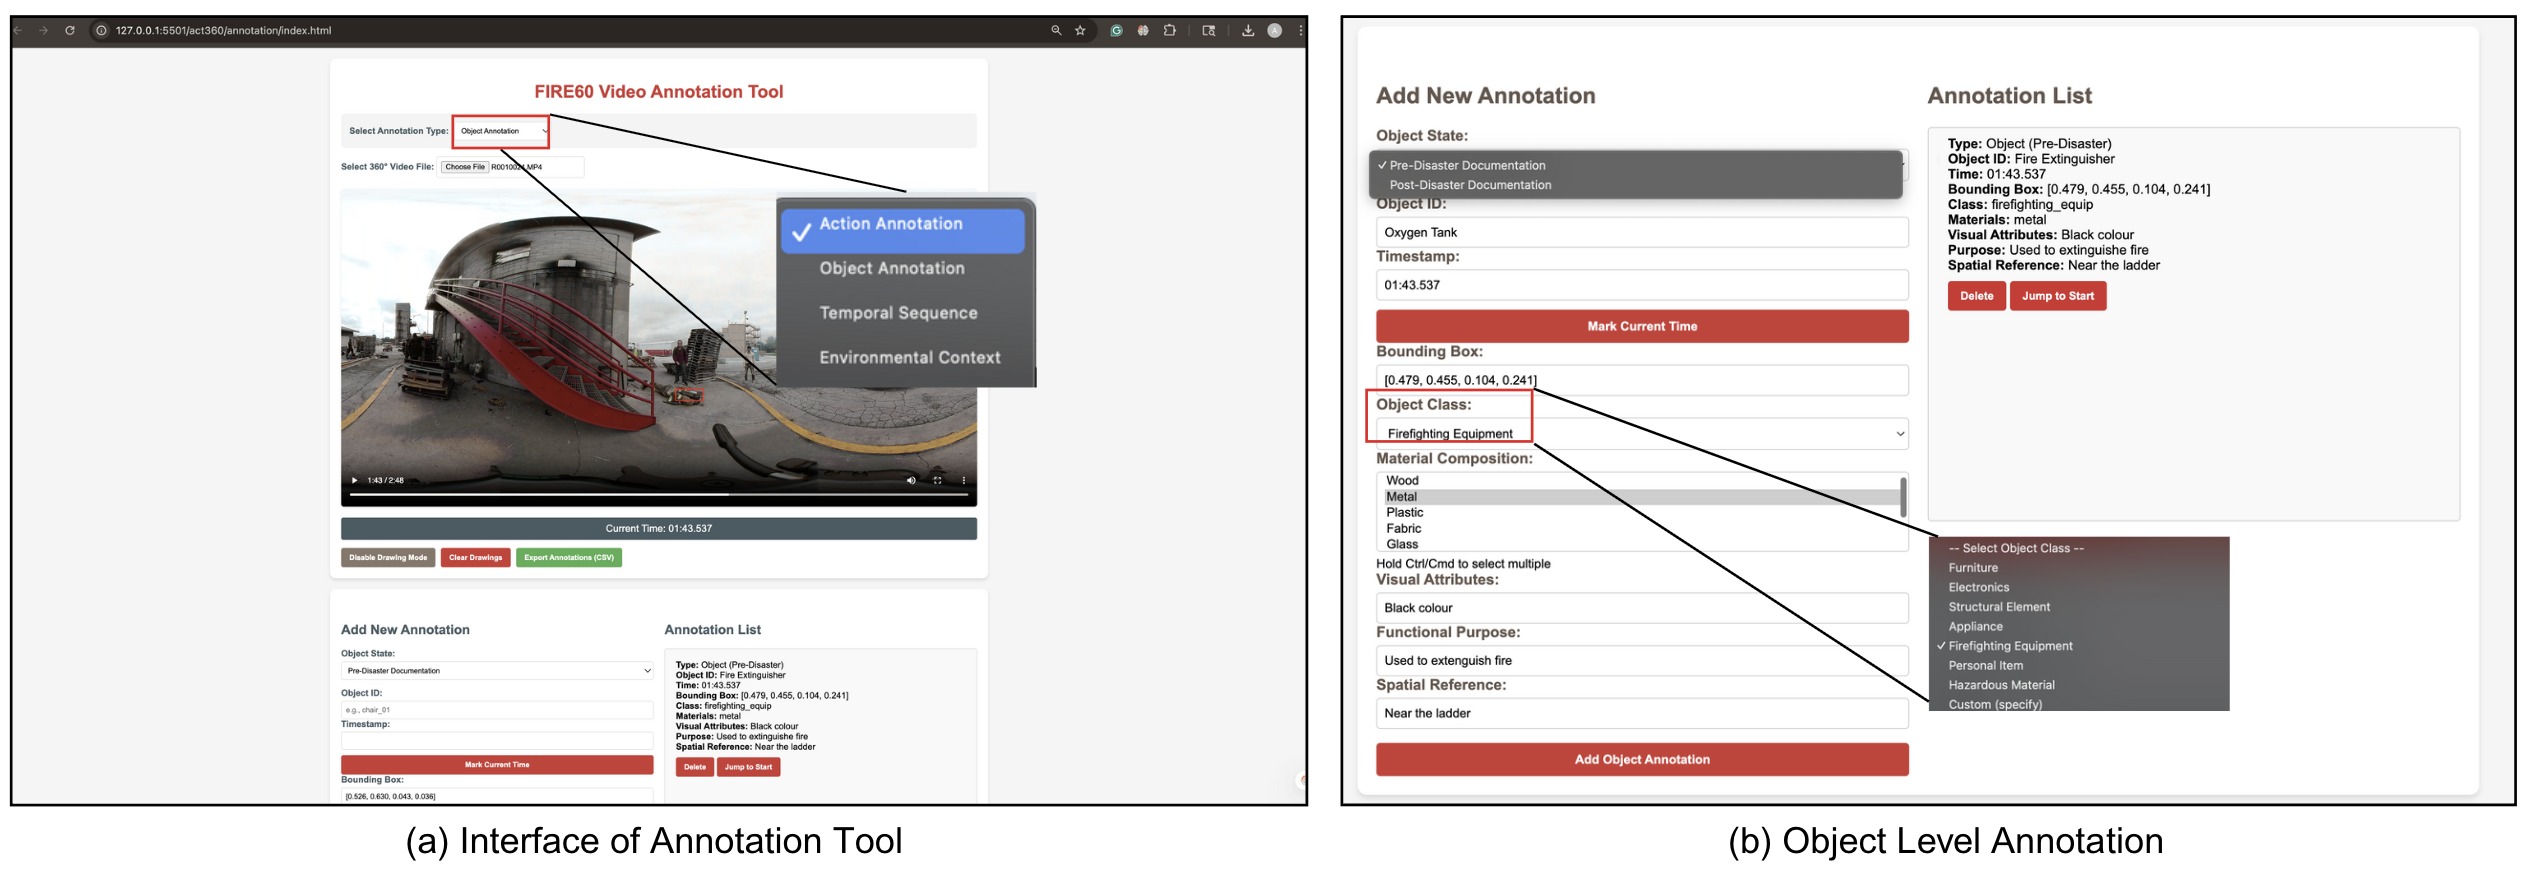}
\caption{Annotation interface for Fire360. (a) The dropdown menu allows annotators to select the annotation type—action, object, temporal sequence, or environmental context. (b) Example of object-level annotation on a video frame, showing bounding box input, object class selection, material composition, spatial reference, and functional attributes.}
\label{fig:annotation_tool_ui}
\end{figure}

\begin{figure}[h]
\centering
\includegraphics[width=\textwidth]{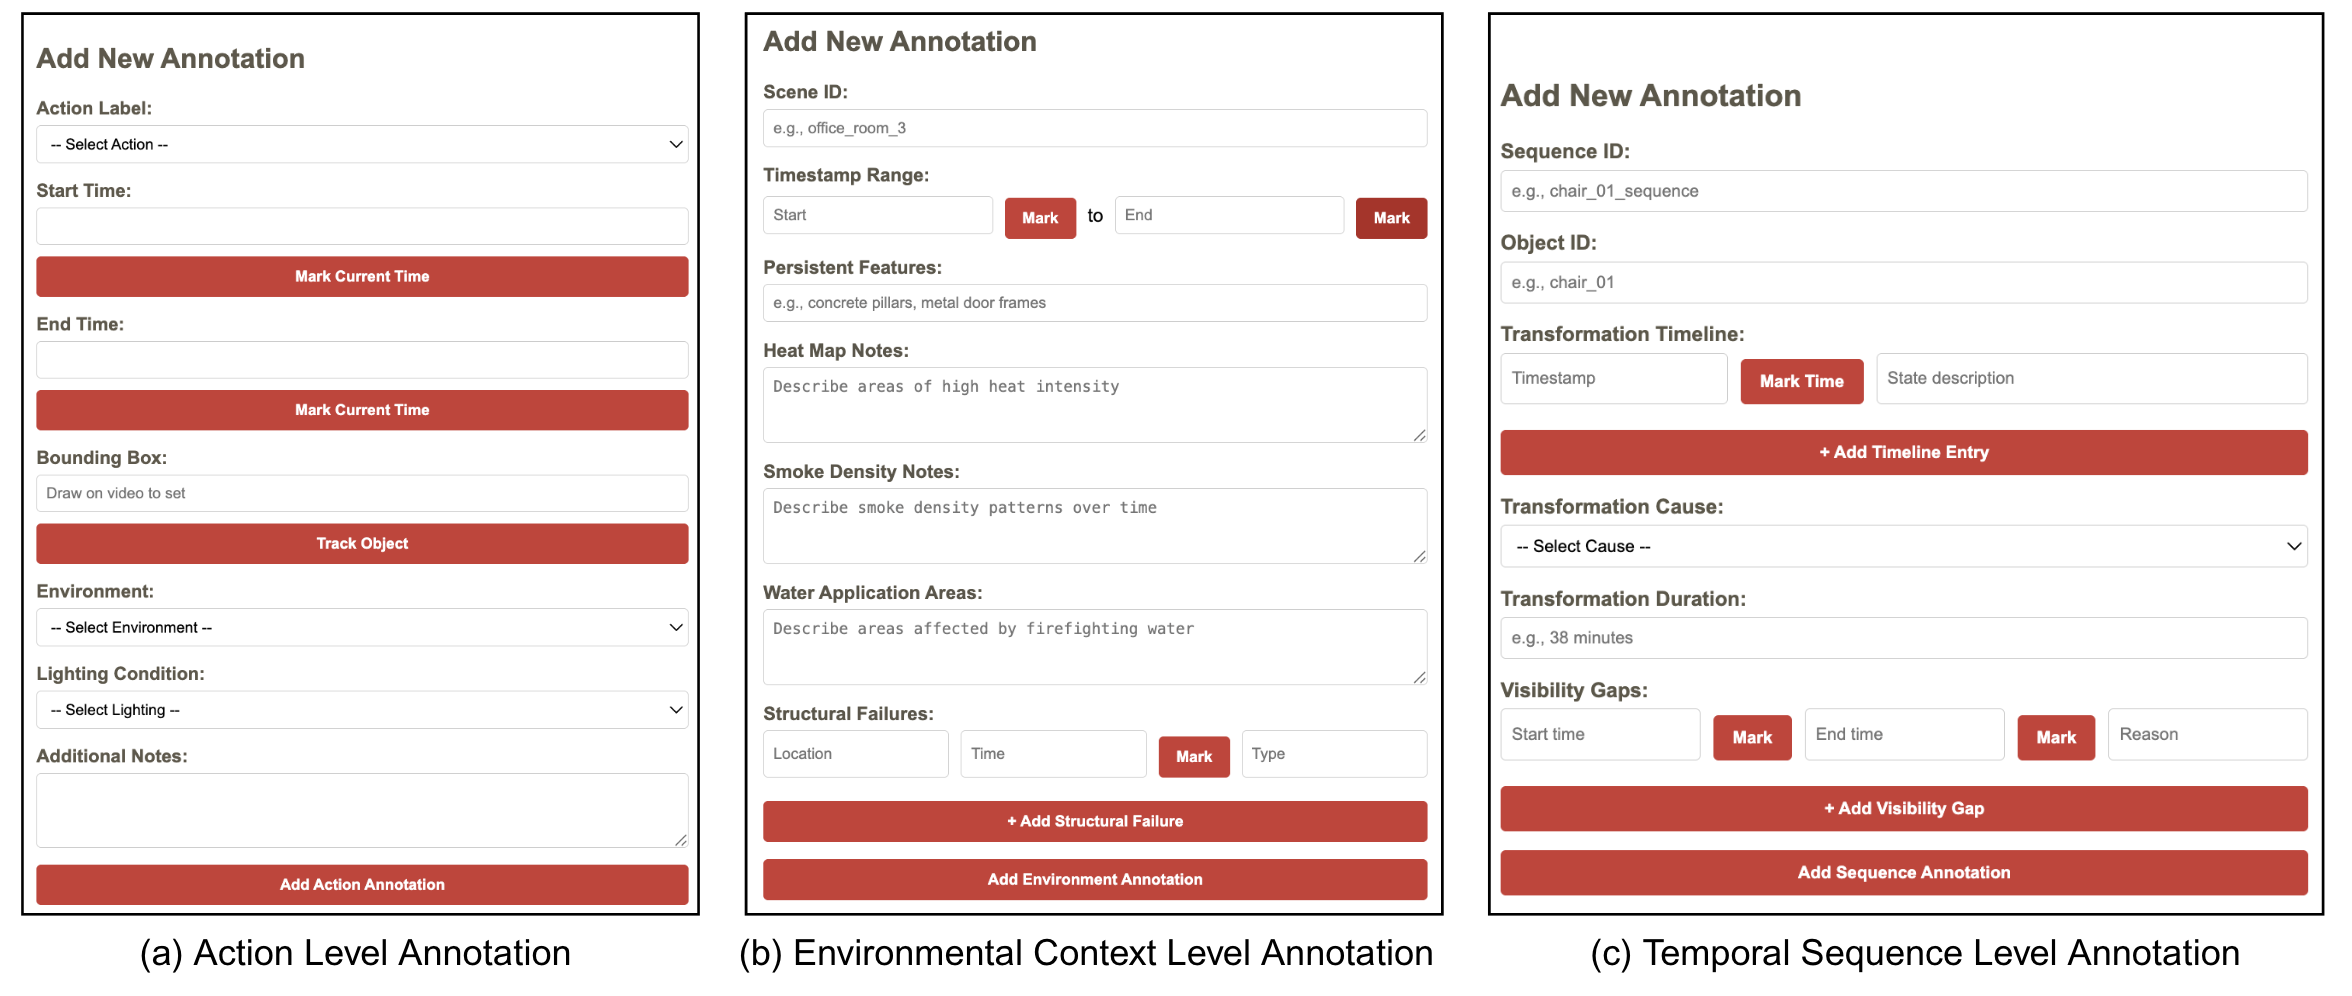}
\caption{Annotation form components for Fire360. (a) Action-level annotation includes temporal boundaries, bounding boxes, and environmental conditions. (b) Environmental context annotation captures persistent features, smoke and heat intensity, structural hazards, and water-affected areas. (c) Temporal sequence annotation enables timeline tracking of object transformations and visibility gaps over extended video segments.}
\label{fig:annotation_modes}
\end{figure}

\textbf{Temporal Action Annotations.}  
Each action label includes timestamps, category, annotator confidence, and optional actor and environment metadata. 
\begin{verbatim}
{
  "action_id": "action_042",
  "start_timestamp": "00:01:45.0",
  "end_timestamp": "00:01:50.5",
  "category": "window_break",
  "confidence_score": 0.92,
  "actors": ["responder_01"],
  "environmental_conditions": {
    "smoke_level": 3,
    "temperature_zone": "high",
    "visibility_rating": "medium"
  }
}
\end{verbatim}

\textit{Spatial Object Annotations.}  
Each object instance is labeled with bounding box coordinates, class, material composition, visibility status, and damage state.
\begin{verbatim}
{
  "object_id": "helmet_023",
  "timestamp": "00:01:35.2",
  "bbox": [420, 260, 75, 80],
  "class": "helmet",
  "material_composition": ["plastic", "metal"],
  "visibility": "smoke_occluded",
  "state": "transformed"
}
\end{verbatim}

\textit{Transformation Tracking.}  
For transformed objects, we track pre/post instances and capture severity, displacement, and residual visual cues.
\begin{verbatim}
{
  "object_id": "hose_015",
  "timestamp": "00:02:12.8",
  "bbox": [300, 180, 50, 60],
  "pre_disaster_id": "hose_015_pre",
  "post_disaster_id": "hose_015_post",
  "transformation": {
    "type": "heat_damage",
    "severity": "extreme",
    "displacement": {"dx": 50, "dy": 20},
    "remaining_features": "charred rubber, partial nozzle visible",
    "difficulty_rating": 5
  }
}
\end{verbatim}

\textit{Environmental Context.}  
Scene-level annotations describe structural layout, temperature gradients, and occlusion conditions.
\begin{verbatim}
{
  "frame_id": "frame_001352",
  "timestamp": "00:02:12.8",
  "room_layout": "hallway",
  "smoke_density": 5,
  "temperature_zones": [
    {"area": "left_wall", "temp": "high"},
    {"area": "ceiling", "temp": "extreme"}
  ],
  "structural_hazards": ["collapsed_ceiling"],
  "visibility_rating": "low"
}
\end{verbatim}

\textbf{Combined Scene Annotation.}  
We support composite entries that integrate all annotation layers for a single frame or video segment.
\begin{verbatim}
{
  "scene_id": "engine_bay_day_001",
  "timestamp": "00:02:12.8",
  "action_annotation": {
    "action_id": "action_043",
    "category": "operating_hose",
    "start_timestamp": "00:02:10.0",
    "end_timestamp": "00:02:20.0",
    "environmental_conditions": {
      "environment": "outdoor_daylight",
      "lighting": "bright"
    },
    "bbox": [430, 220, 110, 140],
    "notes": "Nozzle pointed at smoke source"
  },
  "object_annotation": {
    "object_id": "hose_015",
    "class": "hose",
    "state": "charred",
    "material_composition": ["rubber", "metal"],
    "visibility": "heavily_occluded",
    "visual_attributes": ["flexible", "darkened"],
    "functional_purpose": "water delivery",
    "spatial_reference": "lower left quadrant",
    "bbox": [300, 180, 50, 60]
  },
  "environmental_context": {
    "smoke_level": 5,
    "temperature_zones": [
      {"area": "back_wall", "temp": "extreme", "notes": "Flame zone"}
    ],
    "structural_hazards": [
      {
        "location": "ceiling beam",
        "timestamp": "00:02:05.0",
        "type": "collapse"
      }
    ],
    "water_application_areas": "right quadrant soaked",
    "persistent_features": ["brick wall", "metal post"]
  }
}
\end{verbatim}

\subsection{Qualitative TOR Examples and Prompt Templates}
\label{appendix:qual}

We include qualitative examples to illustrate typical model behaviors and failure cases in the Transformed Object Retrieval (TOR) task. Table~\ref{tab:tor_failure_summary} summarizes model-level accuracy along with the dominant source of error for each method. GPT-4o achieves the highest top-1 accuracy but remains sensitive to distractor regions that resemble the target object. BLIP-2 and CLIP underperform in cases involving material ambiguity and occlusion, respectively.

Figure~\ref{fig:tor_examples} shows three representative cases from the benchmark. The top row depicts a successful retrieval of a helmet with minor damage. In the middle row, the model incorrectly retrieves a metallic pipe that resembles a melted helmet. The bottom row shows a failure case where a charred hose is occluded and not retrieved.

\begin{figure}[t]
\centering
\includegraphics[width=\textwidth]{figures/tor_examples.png}
\caption{Example predictions from the TOR benchmark. Top: successful retrieval (helmet). Middle: distractor error (pipe misclassified as helmet). Bottom: occlusion failure (charred hose not detected).}
\label{fig:tor_examples}
\end{figure}

To support replicability and structured evaluation, we include a set of representative prompts and expected outputs for each benchmark task. These prompt templates guide model behavior in safety reasoning, object retrieval, and spatial understanding under degraded conditions. Table~\ref{tab:prompt_templates} summarizes prompt-response pairs used across tasks such as TOR, Safety Reasoning, and 360$^{\circ}$ VQA.

\begin{table}[t]
\centering
\caption{Sample prompt-response pairs used in Fire360 evaluation.}
\label{tab:prompt_templates}
\footnotesize
\resizebox{\linewidth}{!}{
\begin{tabular}{@{}c@{}}
\begin{tabular}{p{0.28\linewidth}p{0.34\linewidth}p{0.34\linewidth}}
\toprule
\textbf{Task} & \textbf{Prompt} & \textbf{Expected Output} \\
\midrule
TOR & \texttt{Given the pristine helmet, find the degraded region. Rule out pipes.} & \texttt{Degraded helmet, 60\% soot.} \\
Safety Reasoning & \texttt{Is the PPE intact?} & \texttt{Unsafe: Mask unsealed.} \\
VQA & \texttt{Is three-point contact maintained?} & \texttt{Yes, one hand, both feet on rungs.} \\
\bottomrule
\end{tabular}
\end{tabular}
}
\end{table}

% \subsection{Qualitative TOR Examples and Prompt Templates}
% \label{appendix:qual}

% We include qualitative analysis to illustrate typical model behaviors and failure modes in the Transformed Object Retrieval (TOR) task. Table~\ref{tab:tor_failure_summary} summarizes model-level accuracy along with the dominant source of error for each method. GPT-4o achieves the highest top-1 accuracy but remains sensitive to distractor regions that resemble the target object. BLIP-2 and CLIP underperform in cases involving material ambiguity and occlusion, respectively.

% Although images are not included in this version of the appendix, representative TOR cases span three main categories: (1) successful retrievals where the degraded object retains partial structural integrity (e.g., lightly burnt helmets), (2) distractor failures where models confuse structurally similar objects such as pipes and ladders, and (3) occlusion-induced errors where charred or melted objects are partially obscured by smoke or debris.

% To support structured prompting and replicability, we include a set of representative prompts and expected outputs for each benchmark task. These prompt templates guide model behavior in safety reasoning, object retrieval, and spatial understanding under degraded conditions. Table~\ref{tab:prompt_templates} summarizes prompt-response pairs used across tasks such as TOR, Safety Reasoning, and 360$^{\circ}$ VQA.

\subsection{Technical Considerations and Task Justification}
\label{appendix:context}

\textbf{360$^\circ$ Processing Details.}  
All raw videos are recorded in equirectangular format and processed using OpenCV-based tools to generate 90$^\circ$ rectilinear projections. These projections reduce distortion near polar regions while preserving spatial layout and degradation artifacts. No learning-based distortion correction is applied, in order to maintain the fidelity of real-world visual degradations such as smoke, blur, and lens glare.

\textbf{Task Motivation and Relevance.}  
Each benchmark task is grounded in real-world firefighter protocols observed and validated by domain experts. VQA emphasizes spatial awareness (e.g., recognizing PPE compliance or locating safety hazards), while temporal captioning approximates incident summarization—a key requirement in post-incident reporting and training debriefings. Safety Reasoning is modeled on procedural checklists used during real operations, where missing or misclassified safety violations can have critical implications.

\textbf{Domain-Specific Failure Insights.}  
Observed model failures are not uniformly distributed: occlusions from smoke and debris, visual similarity between degraded and intact objects (e.g., pipes vs. melted helmets), and material misclassification (rubber vs. metal) frequently lead to retrieval or reasoning errors. These failure modes mirror real-world firefighting challenges, where visibility is compromised and time-sensitive decisions rely on partial visual cues. The annotated benchmark captures these operational edge cases to enable targeted analysis of model limitations under extreme conditions.
