# Supplementary material for: Fire360: A Benchmark for Robust Perception and Episodic Memory in Degraded 360-Degree Firefighting Videos
Source: arXiv:2506.02167 source file (2025-06-02)
Supplement: Supplementary file 4 [file appendix-D.tex]

\appendix
\section*{Appendix B: Model Setup and Evaluation Protocols}
\label{appendix:setup}
