# Supplementary material for: Fire360: A Benchmark for Robust Perception and Episodic Memory in Degraded 360-Degree Firefighting Videos
Source: arXiv:2506.02167 source file (2025-06-02)
Supplement: Supplementary file 5 [file appendix-E.tex]

\appendix
\section*{Appendix C: Statistical Evaluation and Per-Class Breakdown}
\label{appendix:stats}

% We report 95\% bootstrap confidence intervals (1,000 resamples) for all TOR metrics. Figure~\ref{fig:tor_class_iou} shows classwise top-1 retrieval accuracy and standard error. The benchmark includes 20 firefighter-relevant object categories. Certain rigid objects (e.g., SCBA tanks, helmets) are retrieved more reliably than deformable or heavily occluded ones (e.g., gloves, masks).

% \begin{figure}[h]
% \centering
% \includegraphics[width=0.9\linewidth]{figures/tor_classwise_stats.png}
% \caption{Top-1 retrieval accuracy across 20 object categories in TOR. Error bars show standard error over 1,000 bootstrap resamples.}
% \label{fig:tor_class_iou}
% \end{figure}
