# Supplementary material for: Fire360: A Benchmark for Robust Perception and Episodic Memory in Degraded 360-Degree Firefighting Videos
Source: arXiv:2506.02167 source file (2025-06-02)
Supplement: Supplementary file 6 [file appendix-c.tex]

\appendix
\section*{Appendix A: Qualitative Results and Embedding Comparison}
\label{appendix:qual}
